# Supplementary material for: Age-of-Gradient Updates for Federated Learning over Random Access Channels
Source: arXiv:2410.11986 source file (2024-10-15)
Supplement: Supplementary file 1 [file supplementary_main.tex]

\documentclass[12pt,a4paper]{article}

% Essential Packages
\usepackage{graphicx}
\usepackage{amsmath, amssymb}
\usepackage{hyperref}
\usepackage{geometry}
\geometry{left=2cm,right=2cm,top=2cm,bottom=2cm}
\usepackage[utf8]{inputenc}
\usepackage[english]{babel}
\usepackage{authblk}
\usepackage{xeCJK}
\usepackage{float}
% Figures and Tables
\usepackage{caption}
\usepackage{subcaption}
\usepackage{booktabs}
\usepackage{multirow}

% TikZ and PGFPlots for diagrams and plots
\usepackage{tikz}
\usepackage{pgfplots}
\usetikzlibrary{arrows.meta, positioning, shapes.geometric, backgrounds, pgfplots.fillbetween}
\pgfplotsset{compat=newest}
\appendix

% Title and Author Information
\title{Supplementary Material for \\
``Age-of-Gradient Updates for  Federated Learning over Random Access Channels''}
\author{}
\date{} % Remove the date

\newcommand{\topK}{ {\mathsf{top}}_{\kappa}}
\newcommand{\randK}{ {\mathsf{rand}}_{\kappa}}
\begin{document}
\maketitle

\section{AoG Policy}

In this section, we briefly describe the performance of the AoG policy discussed in Sec. 5 of the main manuscript across various parameters. 

First, we present  a more complete comparison of the performance of the four considered schemes, as is Sec. 6 of the main manuscript: (i) the genie-aided policy, which selects the optimal set of active users 
at each time-frame, (ii) the AoG policy, which uses the magnitude of the user local-gradients as a measure of freshness, (iii) the fix/random policy with $U_A=5$, which selects five active users at random and (iv) the policy in Sec. 4.1 with $U_A=10$ active users.
For the policies with a fix number of active users, we also compare the cases with local memory, $\gamma=1$, versus the cases with no local memory, ie $\gamma=0$.

A few observations on Fig. \ref{fig:matrix fig}.
Generally, $K=5$ provides better performance for the strategies with a variable number of users, while $K=10$ provides better performance for the strategies with a fixed number of users. 
Additionally, error feedback consistently results in a substantial performance improvement, justifying the inherent increase in complexity required to implement this approach.%
Finally, the AoG policy generally performed very close to the genie-aided policy. 
However, it should be noted that the optimization of the policy parameter was performed over a limited number of seeds (five). 

\begin{figure}
\centering    
% Row 1
\begin{tikzpicture}
\begin{axis}[
title = {$U_A=5$},
name=plot1,
ytick pos=left,
width=8.5cm, % Adjust this value to make the plot narrower
height=7cm, % Adjust this value to make the plot shorter
xmin=1, 
xmax=15,
ymin=0.1, 
ymax=0.85,
ytick={0.1,0.2,0.3,0.4,0.5,0.6,0.7,0.8},
legend style={font=\tiny, % Smaller font for the legend
          at={(1,0)}, % Fine-tuned position for the legend
          anchor=south east},
grid=major,
grid style=dashed,
xlabel={Time-frame}, ylabel={Mean Accuracy, $K=5$},
]
\addplot[
            color=red,
        mark=*,
        mark options={scale=0.75},
    ]
    coordinates {
        (1,0.2575)
            (2,0.5069)
            (3,0.6115)
            (4,0.6715)
            (5,0.7046)
            (6,0.7280)
            (7,0.7437)
            (8,0.7559)
            (9,0.7652)
            (10,0.7730)
            (11,0.7794)
            (12,0.7854)
            (13,0.7902)
            (14,0.7949)
            (15,0.7989)
    };
    \addlegendentry{AoG Policy, $\gamma=1$}
    \addplot[
        color=red,
        mark=star,
        dashed
        ]
        coordinates {
        (1,0.344236)
            (2,0.540216)
            (3,0.637048)
            (4,0.68778)
            (5,0.7171)
            (6,0.736684)
            (7,0.751132)
            (8,0.761756)
            (9,0.770292)
            (10,0.777244)
            (11,0.783724)
            (12,0.788796)
            (13,0.793624)
            (14,0.797928)
            (15,0.801668)
        };
        \addlegendentry{Genie-Aided, $\gamma=1$}
        \addplot[
    color=green,
    mark=triangle,
    ]
    coordinates {
    (1,0.1945)
            (2,0.3865)
            (3,0.5135)
            (4,0.5694)
            (5,0.5873)
            (6,0.6370)
            (7,0.6543)
            (8,0.6814)
            (9,0.6798)
            (10,0.7168)
            (11,0.7289)
            (12,0.7396)
            (13,0.7403)
            (14,0.7606)
            (15,0.7745)
    };
    \addlegendentry{$\gamma = 1$}
    \addplot[
        color=blue, mark=triangle,
        ]
        coordinates {
            (1,0.1676)
            (2,0.2322)
            (3,0.2561)
            (4,0.2308)
            (5,0.2152)
            (6,0.2971)
            (7,0.3644)
            (8,0.4104)
            (9,0.5361)
            (10,0.5829)
            (11,0.6117)
            (12,0.6280)
            (13,0.6278)
            (14,0.6402)
            (15,0.6510)
        };
    \addlegendentry{$\gamma=0$}
\end{axis}

\begin{axis}[
title = {$U_A=10$},
name=plot2, at={(plot1.south east)},
ytick=\empty,
width=8.5cm, % Adjust this value to make the plot narrower
height=7cm, % Adjust this value to make the plot shorter
xmin=1, xmax=15,
            ymin=0.1, ymax=0.85,
            ytick=
        {0.1,0.2,0.3,0.4,0.5,0.6,0.7,0.8},
        yticklabels=\empty,
            legend style={font=\tiny, % Smaller font for the legend
                      at={(1,0)}, % Fine-tuned position for the legend
                      anchor=south east},
            grid=major,
            grid style=dashed,
xlabel={Time-frame},
]
\addplot[
        color=red,
        mark=*,
        mark options={scale=0.75},
    ]
    coordinates {
        (1,0.2575)
            (2,0.5069)
            (3,0.6115)
            (4,0.6715)
            (5,0.7046)
            (6,0.7280)
            (7,0.7437)
            (8,0.7559)
            (9,0.7652)
            (10,0.7730)
            (11,0.7794)
            (12,0.7854)
            (13,0.7902)
            (14,0.7949)
            (15,0.7989)
    };
    \addlegendentry{AoG Policy $\gamma=1$}

    \addplot[
        color=red,
        mark=star,
        dashed
        ]
        coordinates {
        (1,0.344236)
            (2,0.540216)
            (3,0.637048)
            (4,0.68778)
            (5,0.7171)
            (6,0.736684)
            (7,0.751132)
            (8,0.761756)
            (9,0.770292)
            (10,0.777244)
            (11,0.783724)
            (12,0.788796)
            (13,0.793624)
            (14,0.797928)
            (15,0.801668)
        };
        \addlegendentry{Genie-Aided $\gamma=1$}
        \addplot[
    color=green,
    mark=triangle,
    ]
    coordinates {
        (1,0.1359)
        (2,0.3643)
        (3,0.4939)
        (4,0.5456)
        (5,0.5733)
        (6,0.6249)
        (7,0.6444)
        (8,0.6717)
        (9,0.6727)
        (10,0.7112)
        (11,0.7262)
        (12,0.7371)
        (13,0.7379)
        (14,0.7589)
        (15,0.7723)
        };
    \addlegendentry{$\gamma = 1$}

    \addplot[
    color=blue, mark=triangle,
    ]
    coordinates {
    (1,0.16602)(2,0.29444)(3,0.36634)(4,0.4654)(5,0.49644)(6,0.51789999)(7,0.56975999)(8,0.59243999)(9,0.6106)(10,0.64545999)(11,0.65754)(12,0.67874001)(13,0.71322001)(14,0.71880001)(15,0.72958001)
    };
    \addlegendentry{$\gamma=0$}
\end{axis}

\end{tikzpicture}

% Row 2
\begin{tikzpicture}
\begin{axis}[
name=plot1,
ytick pos=left,
width=8.5cm, % Adjust this value to make the plot narrower
height=7cm, % Adjust this value to make the plot shorter
xmin=1, xmax=15,
            ymin=0.1, ymax=0.85,
            ytick={0.1,0.2,0.3,0.4,0.5,0.6,0.7,0.8},
            legend style={font=\tiny, % Smaller font for the legend
                      at={(1,0)}, % Fine-tuned position for the legend
                      anchor=south east},
            grid=major,
grid style=dashed,
xlabel={Time-frame}, ylabel={Mean Accuracy, $K=10$},
]
\addplot[
        color=red,
        mark=*,
        mark options={scale=0.75},
    ]
    coordinates {
        (1,0.203096)
            (2,0.392196)
            (3,0.523512)
            (4,0.601912)
            (5,0.645108)
            (6,0.674484)
            (7,0.694136)
            (8,0.70918)
            (9,0.7212)
            (10,0.731032)
            (11,0.73938)
            (12,0.746336)
            (13,0.752236)
            (14,0.757824)
            (15,0.762876)
    };
    \addlegendentry{AoG Policy, $\gamma=1$}

    \addplot[
        color=red,
        mark=star,
        dashed
        ]
        coordinates {
        (1,0.248736)
        (2,0.424724)
        (3,0.547344)
        (4,0.616776)
        (5,0.656220)
        (6,0.682800)
        (7,0.701592)
        (8,0.715752)
        (9,0.727348)
        (10,0.736572)
        (11,0.743692)
        (12,0.750360)
        (13,0.756260)
        (14,0.761064)
        (15,0.765912)
        };
        \addlegendentry{Genie-Aided, $\gamma=1$}
        \addplot[
    color=green,
    mark=triangle,
    ]
    coordinates {
    (1,0.2165924)
        (2,0.378818)
        (3,0.4592748)
        (4,0.5247492)
        (5,0.5943688)
        (6,0.6391516)
        (7,0.680832)
        (8,0.6904988)
        (9,0.7154196)
        (10,0.7269588)
        (11,0.7458832)
        (12,0.7514816)
        (13,0.7596764)
        (14,0.7633252)
        (15,0.7684416)
    };
    \addlegendentry{$\gamma = 1$}
    \addplot[
        color=blue, mark=triangle,
        ]
        coordinates {
        (1,0.2433)(2,0.3602)(3,0.3882)(4,0.4500)(5,0.4897)(6,0.5288)(7,0.5435)(8,0.5643)(9,0.6134)(10,0.6136)(11,0.6705)(12,0.6712)(13,0.6945)(14,0.7241)(15,0.7212)
        };
    \addlegendentry{$\gamma=0$}
\end{axis}

\begin{axis}[
name=plot2, at={(plot1.south east)},
ytick=\empty,
width=8.5cm, % Adjust this value to make the plot narrower
height=7cm, % Adjust this value to make the plot shorter
xmin=1, xmax=15,
            ymin=0.1, ymax=0.85,
            ytick=
        {0.1,0.2,0.3,0.4,0.5,0.6,0.7,0.8},
        yticklabels=\empty,
            legend style={font=\tiny, % Smaller font for the legend
                      at={(1,0)}, % Fine-tuned position for the legend
                      anchor=south east},
            grid=major,
            grid style=dashed,
xlabel={Time-frame},
]
\addplot[
            color=red,
        mark=*,
        mark options={scale=0.75},
    ]
    coordinates {
        (1,0.203096)
            (2,0.392196)
            (3,0.523512)
            (4,0.601912)
            (5,0.645108)
            (6,0.674484)
            (7,0.694136)
            (8,0.70918)
            (9,0.7212)
            (10,0.731032)
            (11,0.73938)
            (12,0.746336)
            (13,0.752236)
            (14,0.757824)
            (15,0.762876)
    };
    \addlegendentry{AoG Policy $\gamma=1$}

    \addplot[
        color=red,
        mark=star,
        dashed
        ]
        coordinates {
        (1,0.248736)
        (2,0.424724)
        (3,0.547344)
        (4,0.616776)
        (5,0.656220)
        (6,0.682800)
        (7,0.701592)
        (8,0.715752)
        (9,0.727348)
        (10,0.736572)
        (11,0.743692)
        (12,0.750360)
        (13,0.756260)
        (14,0.761064)
        (15,0.765912)
        };
        \addlegendentry{Genie-Aided $\gamma=1$}
        \addplot[
    color=green,
    mark=triangle,
    ]
    coordinates {
        (1,0.15423)
        (2,0.3861064)
        (3,0.4542140)
        (4,0.4942888)
        (5,0.5925308)
        (6,0.6247340)
        (7,0.6757796)
        (8,0.6831256)
        (9,0.7135192)
        (10,0.7245312)
        (11,0.7412420)
        (12,0.7499964)
        (13,0.7568760)
        (14,0.7615380)
        (15,0.7669828)
        };
    \addlegendentry{$\gamma = 1$}
    \addplot[
    color=blue, mark=triangle,
    ]
    coordinates {
    (1,0.13046)(2,0.20015999)(3,0.31744)(4,0.36886)(5,0.49866)(6,0.57566)(7,0.60456001)(8,0.6545)(9,0.6897)(10,0.6995)(11,0.7013)(12,0.70316001)(13,0.69516)(14,0.68548)(15,0.69652001)
    };
    \addlegendentry{$\gamma=0$}
\end{axis}

\end{tikzpicture}

% Row 3
\begin{tikzpicture}
\begin{axis}[
name=plot1,
ytick pos=left,
width=8.5cm, % Adjust this value to make the plot narrower
height=7cm, % Adjust this value to make the plot shorter
xmin=1, xmax=15,
            ymin=0.1, ymax=0.85,
            ytick={0.1,0.2,0.3,0.4,0.5,0.6,0.7,0.8},
            legend style={font=\tiny, % Smaller font for the legend
                      at={(1,0)}, % Fine-tuned position for the legend
                      anchor=south east},
            ymajorgrids=false,
            grid=major,
            grid style=dashed,
xlabel={Time-frame}, ylabel={Mean Accuracy, $K=20$},
]
\addplot[
        color=red,
        mark=*,
        mark options={scale=0.75},
    ]
    coordinates {
            (1,0.17204)
            (2,0.271896)
            (3,0.38574)
            (4,0.482352)
            (5,0.549976)
            (6,0.593572)
            (7,0.622956)
            (8,0.644912)
            (9,0.66142)
            (10,0.674712)
            (11,0.686052)
            (12,0.695736)
            (13,0.704076)
            (14,0.7111)
            (15,0.717712)
    };
    \addlegendentry{AoG Policy, 
 $\gamma=1$}

    \addplot[
        color=red,
        mark=star,
        dashed
        ]
        coordinates {
        (1,0.175016)
            (2,0.28178)
            (3,0.40052)
            (4,0.49394)
            (5,0.555612)
            (6,0.595572)
            (7,0.624732)
            (8,0.646068)
            (9,0.662316)
            (10,0.675476)
            (11,0.686768)
            (12,0.696336)
            (13,0.704284)
            (14,0.71336)
            (15,0.717096)
        };
        \addlegendentry{Genie-Aided,  $\gamma=1$}
        \addplot[
    color=green,
    mark=triangle,
    ]
    coordinates {
            (1,0.2087)
            (2,0.3315)
            (3,0.3817)
            (4,0.4300)
            (5,0.4692)
            (6,0.4930)
            (7,0.5139)
            (8,0.6001)
            (9,0.6411)
            (10,0.6596)
            (11,0.6473)
            (12,0.6406)
            (13,0.6467)
            (14,0.6395)
            (15,0.6411)
    };
    \addlegendentry{$\gamma = 1$}
        \addplot[
        color=blue, mark=triangle,
        ]
        coordinates {
        (1, 0.247300)
        (2, 0.298023)
        (3, 0.342007)
        (4, 0.369430)
        (5, 0.424993)
        (6, 0.410617)
        (7, 0.426473)
        (8, 0.478030)
        (9, 0.507600)
        (10, 0.517933)
        (11, 0.508200)
        (12, 0.499877)
        (13, 0.538090)
        (14, 0.557913)
        (15, 0.527680)
        };
    \addlegendentry{$\gamma = 0$}
\end{axis}

\begin{axis}[
name=plot2, at={(plot1.south east)},
ytick=\empty,
width=8.5cm, % Adjust this value to make the plot narrower
height=7cm, % Adjust this value to make the plot shorter
xmin=1, xmax=15,
            ymin=0.1, ymax=0.85,
            ytick=
        {0.1,0.2,0.3,0.4,0.5,0.6,0.7,0.8},
        yticklabels=\empty,
            legend style={font=\tiny, % Smaller font for the legend
                      at={(1,0)}, % Fine-tuned position for the legend
                      anchor=south east},
            grid=major,
            grid style=dashed,
xlabel={Time-frame},
]
\addplot[
            color=red,
        mark=*,
        mark options={scale=0.75},
    ]
    coordinates {
            (1,0.17204)
            (2,0.271896)
            (3,0.38574)
            (4,0.482352)
            (5,0.549976)
            (6,0.593572)
            (7,0.622956)
            (8,0.644912)
            (9,0.66142)
            (10,0.674712)
            (11,0.686052)
            (12,0.695736)
            (13,0.704076)
            (14,0.7111)
            (15,0.717712)
    };
    \addlegendentry{AoG Policy, 
 $\gamma=1$}

    \addplot[
        color=red,
        mark=star,
        dashed
        ]
        coordinates {
        (1,0.175016)
            (2,0.28178)
            (3,0.40052)
            (4,0.49394)
            (5,0.555612)
            (6,0.595572)
            (7,0.624732)
            (8,0.646068)
            (9,0.662316)
            (10,0.675476)
            (11,0.686768)
            (12,0.696336)
            (13,0.704284)
            (14,0.71336)
            (15,0.717096)
        };
        \addlegendentry{Genie-Aided,  $\gamma=1$}
        \addplot[
    color=green,
    mark=triangle,
    ]
    coordinates {
            (1,0.1584)
            (2,0.3513)
            (3,0.4006)
            (4,0.4458)
            (5,0.4997)
            (6,0.5217)
            (7,0.5448)
            (8,0.6292)
            (9,0.6590)
            (10,0.6681)
            (11,0.6747)
            (12,0.6724)
            (13,0.6726)
            (14,0.6739)
            (15,0.6744)
        };
    \addlegendentry{$\gamma = 1$}
    \addplot[
    color=blue, mark=triangle,
    ]
    coordinates {
    (1,0.1802)
            (2,0.3693)
            (3,0.4057)
            (4,0.4457)
            (5,0.4904)
            (6,0.5384)
            (7,0.5383)
            (8,0.5659)
            (9,0.5789)
            (10,0.6079)
            (11,0.6305)
            (12,0.6698)
            (13,0.6898)
            (14,0.6922)
            (15,0.7090)
    };
    \addlegendentry{$\gamma = 0$}
\end{axis}
\end{tikzpicture}

\caption{A comparison of the AoG policy, the genie-aided policy, and the fix/random policy for $U_A=5$ and $U_A=10$. The first row is for $K=5$, the second for $K=10$ and the third for $K=20$. The left column considers the fix/random $U_A=5$, the right one the fix/random for $U_A=10$.}
\label{fig:matrix fig}
\end{figure}

Fig. \ref{fig:threshold policy comparison} provides an alternative perspective on the performance in Fig. \ref{fig:matrix fig}. 
Fig. \ref{fig:threshold policy comparison} highlights that overall better performance can be attained for smaller values of $K$. Intuitively, this suggests that in the considered scenario, the overall diversity among the user performances is relatively low, and thus completeness of the gradients is preferable to diversity.

\begin{figure}
\begin{tikzpicture}
\begin{axis}[
title = {$K=5$},
name=plot1,
ytick pos=left,
width=7cm, % Adjust this value to make the plot narrower
height=7cm, % Adjust this value to make the plot shorter
xmin=1, xmax=15,
            ymin=0.1, ymax=0.85,
            ytick={0.1,0.2,0.3,0.4,0.5,0.6,0.7,0.8},
            legend style={font=\tiny, % Smaller font for the legend
                      at={(1,0)}, % Fine-tuned position for the legend
                      anchor=south east},
            ymajorgrids=false,
            grid=major,
            grid style=dashed,
xlabel={Time-frame}, ylabel={Mean Accuracy},
]
\addplot[
    color=red,
    mark=triangle,
    ]
    coordinates {
        (1,0.1359)
        (2,0.3643)
        (3,0.4939)
        (4,0.5456)
        (5,0.5733)
        (6,0.6249)
        (7,0.6444)
        (8,0.6717)
        (9,0.6727)
        (10,0.7112)
        (11,0.7262)
        (12,0.7371)
        (13,0.7379)
        (14,0.7589)
        (15,0.7723)
        };
    \addlegendentry{fix/random $U_A=10$, $\gamma = 1$}

\addplot[
    color=green,
    mark=o,
    ]
    coordinates {
    (1,0.1945)
            (2,0.3865)
            (3,0.5135)
            (4,0.5694)
            (5,0.5873)
            (6,0.6370)
            (7,0.6543)
            (8,0.6814)
            (9,0.6798)
            (10,0.7168)
            (11,0.7289)
            (12,0.7396)
            (13,0.7403)
            (14,0.7606)
            (15,0.7745)
    };
    \addlegendentry{fix/random $U_A=5$, $\gamma = 1$}

\addplot[
    color=brown, mark=triangle,
    ]
    coordinates {
    (1,0.16602)(2,0.29444)(3,0.36634)(4,0.4654)(5,0.49644)(6,0.51789999)(7,0.56975999)(8,0.59243999)(9,0.6106)(10,0.64545999)(11,0.65754)(12,0.67874001)(13,0.71322001)(14,0.71880001)(15,0.72958001)
    };
    \addlegendentry{fix/random $U_A=10$, $\gamma=0$}

\addplot[
        color=cyan, mark=o,
        ]
        coordinates {
            (1,0.1676)
            (2,0.2322)
            (3,0.2561)
            (4,0.2308)
            (5,0.2152)
            (6,0.2971)
            (7,0.3644)
            (8,0.4104)
            (9,0.5361)
            (10,0.5829)
            (11,0.6117)
            (12,0.6280)
            (13,0.6278)
            (14,0.6402)
            (15,0.6510)
        };
    \addlegendentry{fix/random $U_A=5$, $\gamma=0$}

\addplot[
            color=blue,
        mark=*,
        mark options={scale=0.75},
    ]
    coordinates {
        (1,0.2575)
            (2,0.5069)
            (3,0.6115)
            (4,0.6715)
            (5,0.7046)
            (6,0.7280)
            (7,0.7437)
            (8,0.7559)
            (9,0.7652)
            (10,0.7730)
            (11,0.7794)
            (12,0.7854)
            (13,0.7902)
            (14,0.7949)
            (15,0.7989)
    };
    \addlegendentry{AoG Policy $\gamma=1$}

    \addplot[
        color=purple,
        mark=star,
        thick
        ]
        coordinates {
        (1,0.344236)
            (2,0.540216)
            (3,0.637048)
            (4,0.68778)
            (5,0.7171)
            (6,0.736684)
            (7,0.751132)
            (8,0.761756)
            (9,0.770292)
            (10,0.777244)
            (11,0.783724)
            (12,0.788796)
            (13,0.793624)
            (14,0.797928)
            (15,0.801668)
        };
        \addlegendentry{Genie-Aided $\gamma=1$}
 \end{axis}

\begin{axis}[
title={$K=10$},
name=plot2, at={(plot1.south east)},
ytick=\empty,
width=7cm, % Adjust this value to make the plot narrower
height=7cm, % Adjust this value to make the plot shorter
xmin=1, xmax=15,
            ymin=0.1, ymax=0.85,
            ytick=
        {0.1,0.2,0.3,0.4,0.5,0.6,0.7,0.8},
        yticklabels=\empty,
            legend style={font=\tiny, % Smaller font for the legend
                      at={(1,0)}, % Fine-tuned position for the legend
                      anchor=south east},
            grid=major,
            grid style=dashed,
xlabel={Time-frame},
]
\addplot[
    color=red,
    mark=triangle,
    ]
    coordinates {
        (1,0.15423)
        (2,0.3861064)
        (3,0.4542140)
        (4,0.4942888)
        (5,0.5925308)
        (6,0.6247340)
        (7,0.6757796)
        (8,0.6831256)
        (9,0.7135192)
        (10,0.7245312)
        (11,0.7412420)
        (12,0.7499964)
        (13,0.7568760)
        (14,0.7615380)
        (15,0.7669828)
        };
    \addlegendentry{fix/random $U_A=10$, $\gamma = 1$}

\addplot[
    color=green,
    mark=o,
    ]
    coordinates {
    (1,0.2165924)
        (2,0.378818)
        (3,0.4592748)
        (4,0.5247492)
        (5,0.5943688)
        (6,0.6391516)
        (7,0.680832)
        (8,0.6904988)
        (9,0.7154196)
        (10,0.7269588)
        (11,0.7458832)
        (12,0.7514816)
        (13,0.7596764)
        (14,0.7633252)
        (15,0.7684416)
    };
    \addlegendentry{fix/random $U_A=5$, $\gamma = 1$}

\addplot[
    color=brown, mark=triangle,
    ]
    coordinates {
    (1,0.13046)(2,0.20015999)(3,0.31744)(4,0.36886)(5,0.49866)(6,0.57566)(7,0.60456001)(8,0.6545)(9,0.6897)(10,0.6995)(11,0.7013)(12,0.70316001)(13,0.69516)(14,0.68548)(15,0.69652001)
    };
    \addlegendentry{fix/random $U_A=10$, $\gamma=0$}

\addplot[
        color=cyan, mark=o,
        ]
        coordinates {
        (1,0.2433)(2,0.3602)(3,0.3882)(4,0.4500)(5,0.4897)(6,0.5288)(7,0.5435)(8,0.5643)(9,0.6134)(10,0.6136)(11,0.6705)(12,0.6712)(13,0.6945)(14,0.7241)(15,0.7212)
        };
    \addlegendentry{fix/random $U_A=5$, $\gamma=0$}

\addplot[
        color=blue,
        mark=*,
        mark options={scale=0.75},
    ]
    coordinates {
        (1,0.203096)
            (2,0.392196)
            (3,0.523512)
            (4,0.601912)
            (5,0.645108)
            (6,0.674484)
            (7,0.694136)
            (8,0.70918)
            (9,0.7212)
            (10,0.731032)
            (11,0.73938)
            (12,0.746336)
            (13,0.752236)
            (14,0.757824)
            (15,0.762876)
    };
    \addlegendentry{AoG Policy $\gamma=1$}

    \addplot[
        color=purple,
        mark=star,
        thick
        ]
        coordinates {
        (1,0.248736)
        (2,0.424724)
        (3,0.547344)
        (4,0.616776)
        (5,0.656220)
        (6,0.682800)
        (7,0.701592)
        (8,0.715752)
        (9,0.727348)
        (10,0.736572)
        (11,0.743692)
        (12,0.750360)
        (13,0.756260)
        (14,0.761064)
        (15,0.765912)
        };
        \addlegendentry{Genie-Aided $\gamma=1$}
 \end{axis}

\begin{axis}[
title={$K=20$},
name=plot3, at={(plot2.south east)},
ytick=\empty,
width=7cm, % Adjust this value to make the plot narrower
height=7cm, % Adjust this value to make the plot shorter
xmin=1, xmax=15,
            ymin=0.1, ymax=0.85,
            ytick=
        {0.1,0.2,0.3,0.4,0.5,0.6,0.7,0.8},
        yticklabels=\empty,
            legend style={font=\tiny, % Smaller font for the legend
                      at={(1,0)}, % Fine-tuned position for the legend
                      anchor=south east},
            grid=major,
            grid style=dashed,
xlabel={Time-frame},
]
\addplot[
    color=red,
    mark=triangle,
    ]
    coordinates {
            (1,0.1584)
            (2,0.3513)
            (3,0.4006)
            (4,0.4458)
            (5,0.4997)
            (6,0.5217)
            (7,0.5448)
            (8,0.6292)
            (9,0.6590)
            (10,0.6681)
            (11,0.6747)
            (12,0.6724)
            (13,0.6726)
            (14,0.6739)
            (15,0.6744)
        };
    \addlegendentry{fix/random $U_A=10$, $\gamma = 1$}

\addplot[
    color=green,
    mark=o,
    ]
    coordinates {
            (1,0.2087)
            (2,0.3315)
            (3,0.3817)
            (4,0.4300)
            (5,0.4692)
            (6,0.4930)
            (7,0.5139)
            (8,0.6001)
            (9,0.6411)
            (10,0.6596)
            (11,0.6473)
            (12,0.6406)
            (13,0.6467)
            (14,0.6395)
            (15,0.6411)
    };
    \addlegendentry{fix/random $U_A=5$, $\gamma = 1$}

\addplot[
    color=brown, mark=triangle,
    ]
    coordinates {
    (1,0.1802)
            (2,0.3693)
            (3,0.4057)
            (4,0.4457)
            (5,0.4904)
            (6,0.5384)
            (7,0.5383)
            (8,0.5659)
            (9,0.5789)
            (10,0.6079)
            (11,0.6305)
            (12,0.6698)
            (13,0.6898)
            (14,0.6922)
            (15,0.7090)
    };
    \addlegendentry{fix/random $U_A=10$, $\gamma = 0$}

\addplot[
        color=cyan, mark=o,
        ]
        coordinates {
        (1, 0.247300)
        (2, 0.298023)
        (3, 0.342007)
        (4, 0.369430)
        (5, 0.424993)
        (6, 0.410617)
        (7, 0.426473)
        (8, 0.478030)
        (9, 0.507600)
        (10, 0.517933)
        (11, 0.508200)
        (12, 0.499877)
        (13, 0.538090)
        (14, 0.557913)
        (15, 0.527680)
        };
    \addlegendentry{fix/random $U_A=5$, $\gamma = 0$}

\addplot[
            color=blue,
        mark=*,
        mark options={scale=0.75},
    ]
    coordinates {
            (1,0.17204)
            (2,0.271896)
            (3,0.38574)
            (4,0.482352)
            (5,0.549976)
            (6,0.593572)
            (7,0.622956)
            (8,0.644912)
            (9,0.66142)
            (10,0.674712)
            (11,0.686052)
            (12,0.695736)
            (13,0.704076)
            (14,0.7111)
            (15,0.717712)
    };
    \addlegendentry{AoG Policy}

    \addplot[
        color=purple,
        mark=star,
        thick
        ]
        coordinates {
        (1,0.175016)
            (2,0.28178)
            (3,0.40052)
            (4,0.49394)
            (5,0.555612)
            (6,0.595572)
            (7,0.624732)
            (8,0.646068)
            (9,0.662316)
            (10,0.675476)
            (11,0.686768)
            (12,0.696336)
            (13,0.704284)
            (14,0.71336)
            (15,0.717096)
        };
        \addlegendentry{Genie-Aided $\gamma=1$}
 \end{axis}
\end{tikzpicture}
\caption{The overall comparison of baseline and the proposed methods for various values of $K$: $K=5$ in the left panel, $K=10$ in the central one, and $K=20$ in the right one.}
\label{fig:threshold policy comparison}
\end{figure}

% \newpage
% \section{Gradient Magnitude}

\newpage
\section{Error Feedback Strategy}
In the main manuscript, in Sec. 6  and in Fig. 5, we have chosen the memory(forget) coefficient as $\gamma=1$ for the AoG policy as well as the genie-aided policy.
Numerical experimentation has shown that a choice of the $\gamma \in [0.7, 1]$ has a good overall performance. 
In Fig. \ref{fig:forget coefficient} we plot the accuracy attained at each time-frame for a range of $\gamma \in [0.1,1]$ for the scenario in Sec. 4.1.
While $\gamma=0.7$ and $\gamma=0.5$ perform well in the scenario in which all users contend for the channel transmission, the value $\gamma=1$ performs better in the Genie-Aided policy: this is shown in Fig. \ref{fig:gamma compare(0.6 included)}.

\begin{figure}[H]
    \centering
    
\begin{tikzpicture}
\begin{axis}[
    title={Forget Coefficient's Effect on Global Model},
    width=9cm, % Adjust this value to make the plot narrower
    height=7cm, % Adjust this value to make the plot shorter
    xlabel={Time-frame},
    ylabel={Mean Accuracy},
    xmin=1, xmax=10,
    ymin=0, ymax=0.8,
    xtick={1,2,3,4,5,6,7,8,9,10},
    ytick={0,0.1,0.2,0.3,0.4,0.5,0.6,0.7,0.8},
    legend pos=south east,
    legend style={font=\scriptsize},
    ymajorgrids=true,
    grid style=dashed,
]

\addplot[
    color=blue,
    mark=square,
    ]
    coordinates {
    (1,0.1203)(2,0.18366)(3,0.22948)(4,0.34462)(5,0.40506001)(6,0.47831999)(7,0.53593999)(8,0.60862)(9,0.67175999)(10,0.68572)
    };
    \addlegendentry{$\gamma = 1.0$}

\addplot[
    color=red,
    mark=o,
    ]
    coordinates {
    (1,0.15224)(2,0.17268)(3,0.26326)(4,0.35171999)(5,0.40778)(6,0.46055999)(7,0.57568001)(8,0.63923999)(9,0.66498)(10,0.68728001)
    };
    \addlegendentry{$\gamma = 0.9$}

\addplot[
    color=green,
    mark=triangle,
    ]
    coordinates {
    (1,0.172)(2,0.26512)(3,0.29352)(4,0.37668)(5,0.41154001)(6,0.48220001)(7,0.57934001)(8,0.64543999)(9,0.67116001)(10,0.70419999)
    };
    \addlegendentry{$\gamma = 0.8$}

\addplot[
    color=purple,
    mark=diamond,
    ]
    coordinates {
    (1,0.14488)(2,0.2273)(3,0.40222001)(4,0.476)(5,0.50310001)(6,0.53612)(7,0.60161999)(8,0.65086001)(9,0.68396001)(10,0.7187)
    };
    \addlegendentry{$\gamma = 0.7$}

\addplot[
    color=orange,
    mark=star,
    ]
    coordinates {
    (1,0.15186)(2,0.18372)(3,0.3951)(4,0.43534)(5,0.50091999)(6,0.55848)(7,0.64794001)(8,0.66578)(9,0.68296)(10,0.70422)
    };
    \addlegendentry{$\gamma = 0.5$}

\addplot[
    color=brown,
    mark=x,
    ]
    coordinates {
    (1,0.11818)(2,0.13404)(3,0.22374)(4,0.29995999)(5,0.33895999)(6,0.39022001)(7,0.51330001)(8,0.5969)(9,0.64424001)(10,0.66108)
    };
    \addlegendentry{ $\gamma = 0.1$}
\end{axis}
\end{tikzpicture}
\caption{The accuracy per time-frame for various forget coefficients in (8): $\gamma \in \{0.1, 0.5, 0.7, 0.8, 0.9, 1\}$. }
\label{fig:forget coefficient}
\end{figure}

\begin{figure}
    \centering
    
\begin{tikzpicture}
\begin{axis}[
    title={$K=10$},
    width=9cm, % Adjust this value to make the plot narrower
    height=7cm, % Adjust this value to make the plot shorter
    xlabel={Time-frame},
    ylabel={Mean Accuracy},
    xmin=1, xmax=15,
    ymin=0, ymax=0.85,
    xtick={1,2,3,4,5,6,7,8,9,10,11,12,13,14,15},
    ytick={0,0.1,0.2,0.3,0.4,0.5,0.6,0.7,0.8},
    legend pos=south east,
    legend style={font=\scriptsize},
    ymajorgrids=true,
    grid style=dashed,
]

\addplot[color=orange, mark=diamond] coordinates {
        (1, 0.21543734)
        (2, 0.35440512)
        (3, 0.41964904)
        (4, 0.49021966)
        (5, 0.52444324)
        (6, 0.55481194)
        (7, 0.61745004)
        (8, 0.6595054)
        (9, 0.67657006)
        (10, 0.68478636)
        (11, 0.6924799)
        (12, 0.69918556)
        (13, 0.72599702)
        (14, 0.7387599)
        (15, 0.74435536)
    };
    \addlegendentry{Genie-Aided $\gamma=0$}
\addplot[color=blue, mark=o] coordinates {
        (1, 0.2110218)
        (2, 0.3463514)
        (3, 0.329725733333333)
        (4, 0.3264128)
        (5, 0.4684284)
        (6, 0.510068266666667)
        (7, 0.555312733333334)
        (8, 0.584628133333333)
        (9, 0.604379533333333)
        (10, 0.656001333333333)
        (11, 0.674250266666667)
        (12, 0.691209266666667)
        (13, 0.709120666666667)
        (14, 0.7235208)
        (15, 0.730675)
    };
    \addlegendentry{Genie-Aided $\gamma=0.6$}
    \addplot[
        color=purple,
        mark=star,
        thick
        ]
        coordinates {
        (1,0.248736)
        (2,0.424724)
        (3,0.547344)
        (4,0.616776)
        (5,0.656220)
        (6,0.682800)
        (7,0.701592)
        (8,0.715752)
        (9,0.727348)
        (10,0.736572)
        (11,0.743692)
        (12,0.750360)
        (13,0.756260)
        (14,0.761064)
        (15,0.765912)
        };
        \addlegendentry{Genie-Aided $\gamma=1$}
\end{axis}
\end{tikzpicture}
\caption{The accuracy per time-frame for three different forget coefficients.}
\label{fig:gamma compare(0.6 included)}
\end{figure}

\newpage
\section{Gradient Sparsification Strategy}
Another ingredient of the AoG strategy introduced in Sec. 4.1 and Sec. 5 is the gradient sparsification using $\topK$.
In Fig. \ref{fig:sparsification strategy compare} we present simulation results from Sec. 4.1 using both $\topK$ or $\randK$ for various values of $K$ ($K=5$, $10$, $15$ or $20$).  
These results validate the choice of $\topK$ as a well-performing gradient compression strategy for the RACH-FL model.

% Figure for Rand-K vs Top-K
\begin{figure}[H]
    \centering
\begin{tikzpicture}
\begin{axis}[
    title={Genie-Aided Policy $K=5,10,15,20$},
    width=11cm, % Adjust this value to make the plot narrower
    height=9cm, % Adjust this value to make the plot shorter
    xlabel={Time-frame},
    ylabel={Mean Accuracy},
    xmin=1, xmax=15,
    ymin=0, ymax=0.85,
    xtick={1,2,3,4,5,6,7,8,9,10,11,12,13,14,15},
    ytick={0,0.1,0.2,0.3,0.4,0.5,0.6,0.7,0.8},
    legend pos=south east,
    legend style={font=\scriptsize},
    ymajorgrids=true,
    grid style=dashed,
]

\addplot[
        color=purple,
        mark=star,
        dashed
        ]
        coordinates {
        (1,0.344236)
            (2,0.540216)
            (3,0.637048)
            (4,0.68778)
            (5,0.7171)
            (6,0.736684)
            (7,0.751132)
            (8,0.761756)
            (9,0.770292)
            (10,0.777244)
            (11,0.783724)
            (12,0.788796)
            (13,0.793624)
            (14,0.797928)
            (15,0.801668)
        };
        \addlegendentry{$K=5$, $\topK$}
\addplot[color=purple, mark=*] coordinates {
        (1, 0.163364)
        (2, 0.256404)
        (3, 0.361004)
        (4, 0.451444)
        (5, 0.517732)
        (6, 0.5653)
        (7, 0.600064)
        (8, 0.62634)
        (9, 0.646784)
        (10, 0.663664)
        (11, 0.677596)
        (12, 0.689372)
        (13, 0.699664)
        (14, 0.7085)
        (15, 0.716816)
    };
     \addlegendentry{$K=5$, $\randK$}   
\addplot[
        color=blue,
        mark=star,
        dashed
        ]
        coordinates {
        (1,0.248736)
        (2,0.424724)
        (3,0.547344)
        (4,0.616776)
        (5,0.656220)
        (6,0.682800)
        (7,0.701592)
        (8,0.715752)
        (9,0.727348)
        (10,0.736572)
        (11,0.743692)
        (12,0.750360)
        (13,0.756260)
        (14,0.761064)
        (15,0.765912)
        };
        \addlegendentry{$K=10$, $\topK$}
\addplot[color=blue, mark=*] coordinates {
        (1, 0.128396)
        (2, 0.161876)
        (3, 0.204344)
        (4, 0.254524)
        (5, 0.308128)
        (6, 0.361756)
        (7, 0.411432)
        (8, 0.454544)
        (9, 0.490432)
        (10, 0.520312)
        (11, 0.546124)
        (12, 0.568384)
        (13, 0.58678)
        (14, 0.602496)
        (15, 0.616416)
    };
    \addlegendentry{$K=10$, $\randK$}
\addplot[color=orange, mark=star, dashed] coordinates {
        (1, 0.201745)
        (2, 0.339875)
        (3, 0.46722)
        (4, 0.55309)
        (5, 0.604635)
        (6, 0.637805)
        (7, 0.66045)
        (8, 0.67746)
        (9, 0.69138)
        (10, 0.703075)
        (11, 0.712885)
        (12, 0.72073)
        (13, 0.72747)
        (14, 0.733525)
        (15, 0.739005)
    };
    \addlegendentry{$K=15$, $\topK$}
\addplot[color=orange, mark=*] coordinates {
        (1, 0.11866)
        (2, 0.137632)
        (3, 0.161276)
        (4, 0.188456)
        (5, 0.21926)
        (6, 0.252432)
        (7, 0.289024)
        (8, 0.325148)
        (9, 0.360904)
        (10, 0.394596)
        (11, 0.42598)
        (12, 0.454232)
        (13, 0.479556)
        (14, 0.501456)
        (15, 0.521256)
    };
    \addlegendentry{$K=15$, $\randK$}
\addplot[
        color=red,
        mark=star,
        dashed
        ]
        coordinates {
        (1,0.175016)
            (2,0.28178)
            (3,0.40052)
            (4,0.49394)
            (5,0.555612)
            (6,0.595572)
            (7,0.624732)
            (8,0.646068)
            (9,0.662316)
            (10,0.675476)
            (11,0.686768)
            (12,0.696336)
            (13,0.704284)
            (14,0.71336)
            (15,0.717096)
        };
        \addlegendentry{$K=20$, $\topK$}
\addplot[color=red, mark=*] coordinates {
        (1, 0.114332)
        (2, 0.127524)
        (3, 0.1427)
        (4, 0.160812)
        (5, 0.18052)
        (6, 0.202344)
        (7, 0.226144)
        (8, 0.251328)
        (9, 0.278268)
        (10, 0.305708)
        (11, 0.332548)
        (12, 0.3596)
        (13, 0.38578)
        (14, 0.410228)
        (15, 0.432344)
    };
    \addlegendentry{$K=20$, $\randK$}
\end{axis}
\end{tikzpicture}
\caption{The accuracy per time-frame for two different sparsification strategy. All of which uses $\gamma=1$, with the genie-aided policy.}
\label{fig:sparsification strategy compare}
\end{figure}

\end{document}
